# Supplementary material for: Meta-Learning an In-Context Transformer Model of Human Higher Visual Cortex
Source: arXiv:2505.15813 source file (2025-11-17)

True  $t$ -statistics

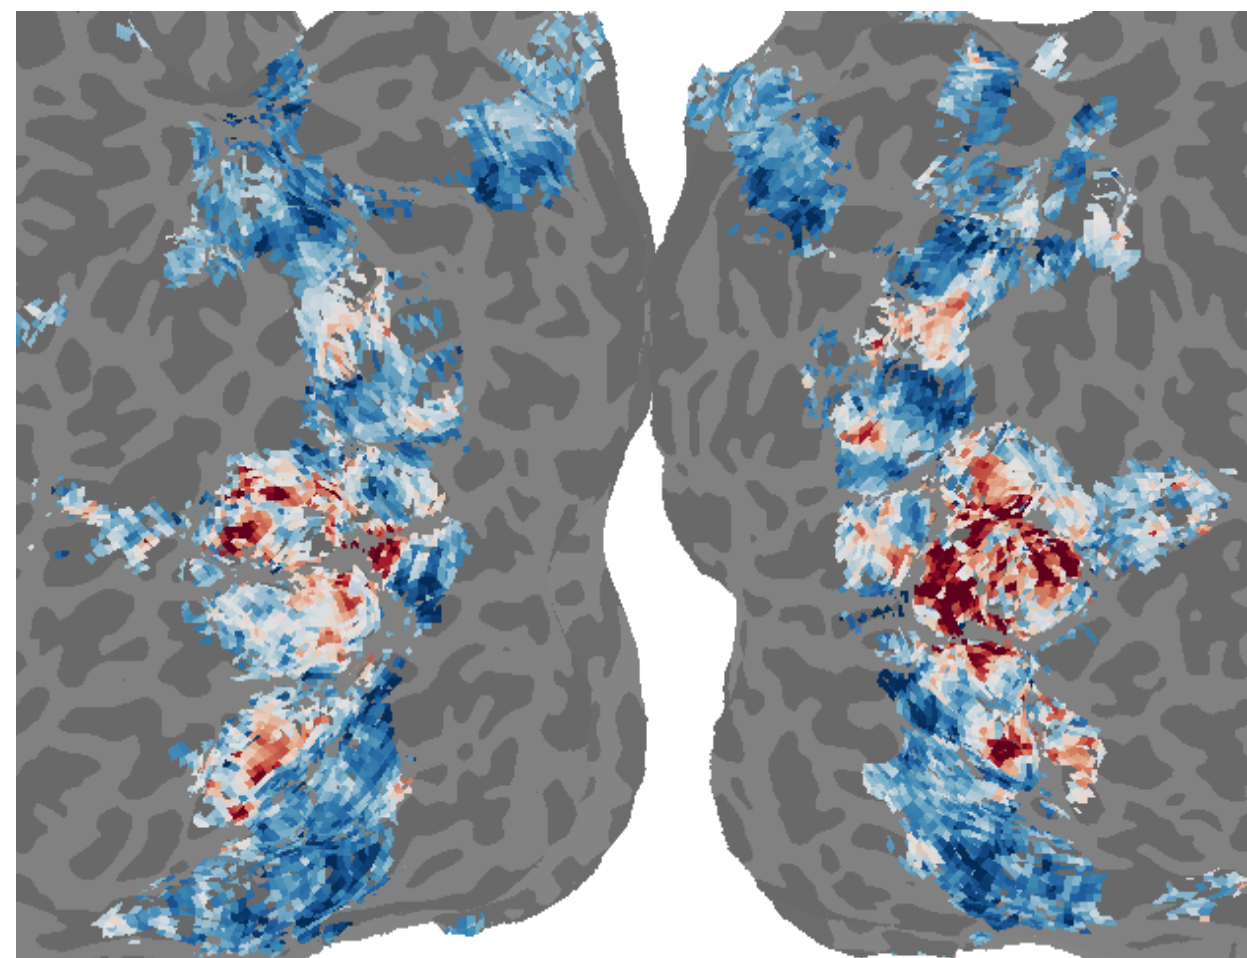

$vmin$

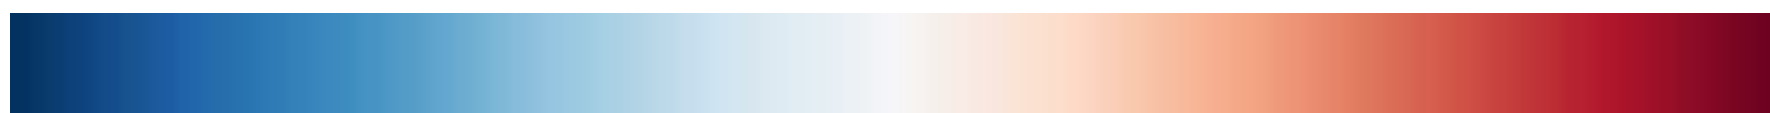

$vmax$

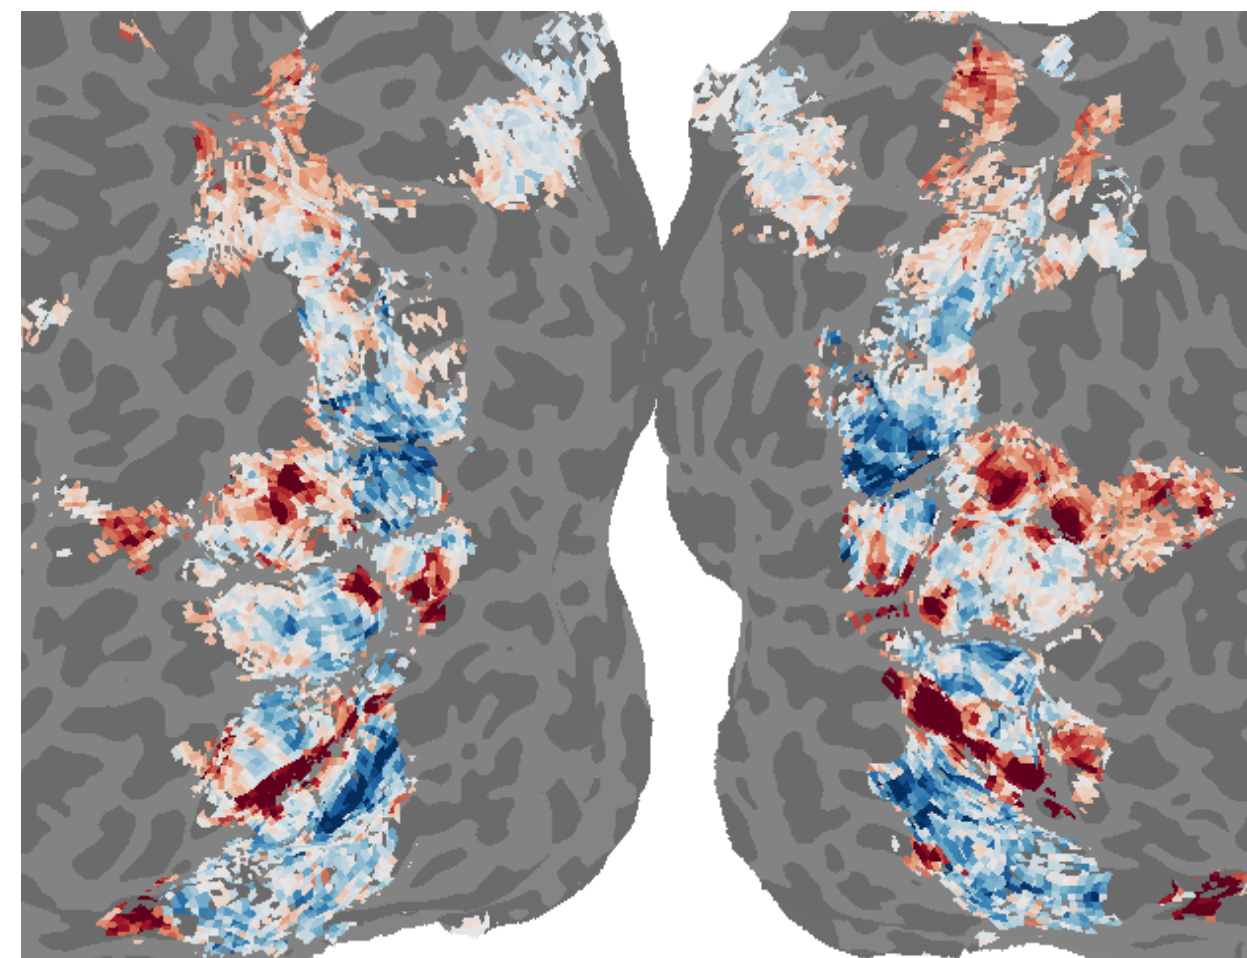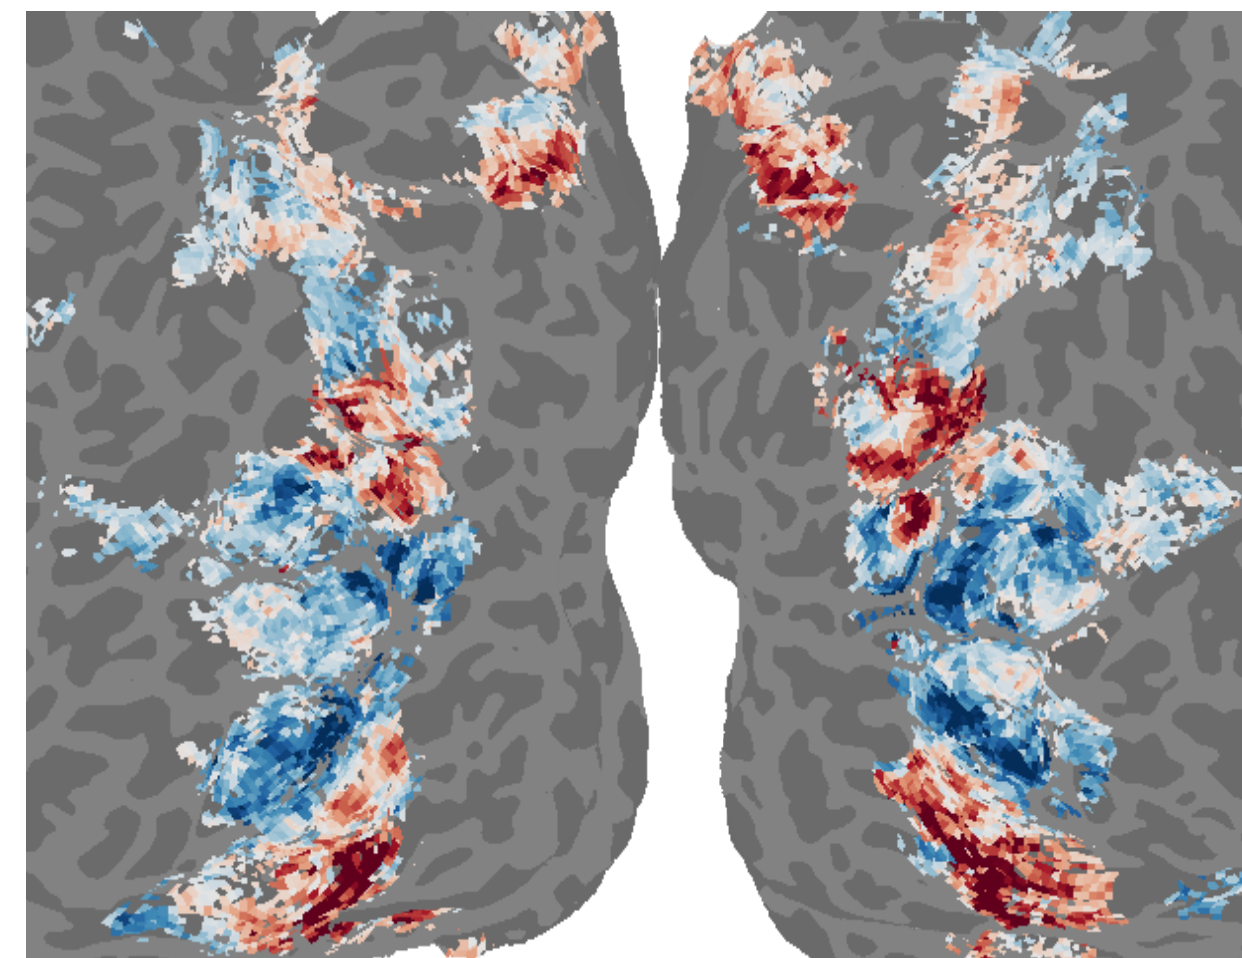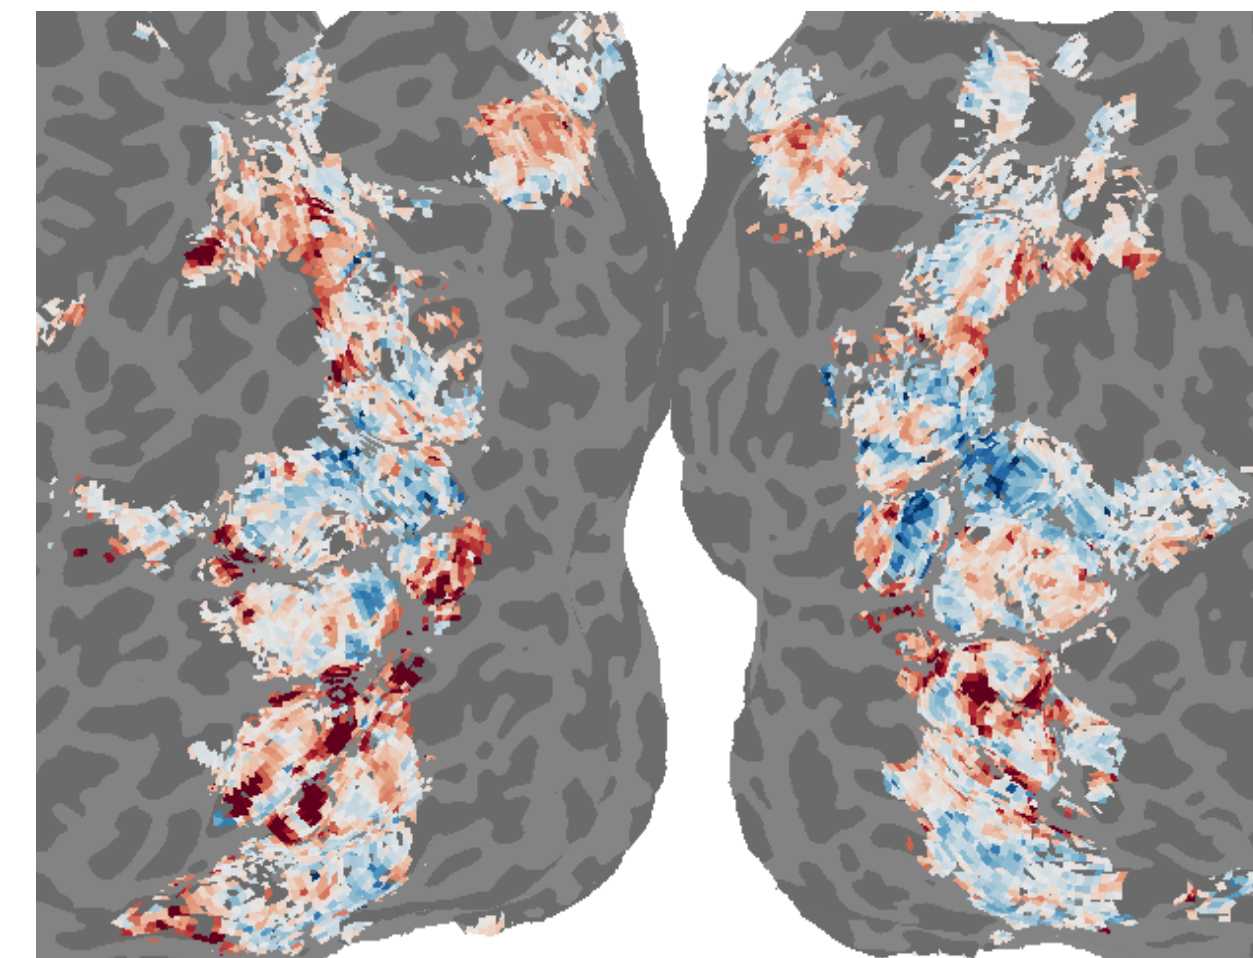

probing

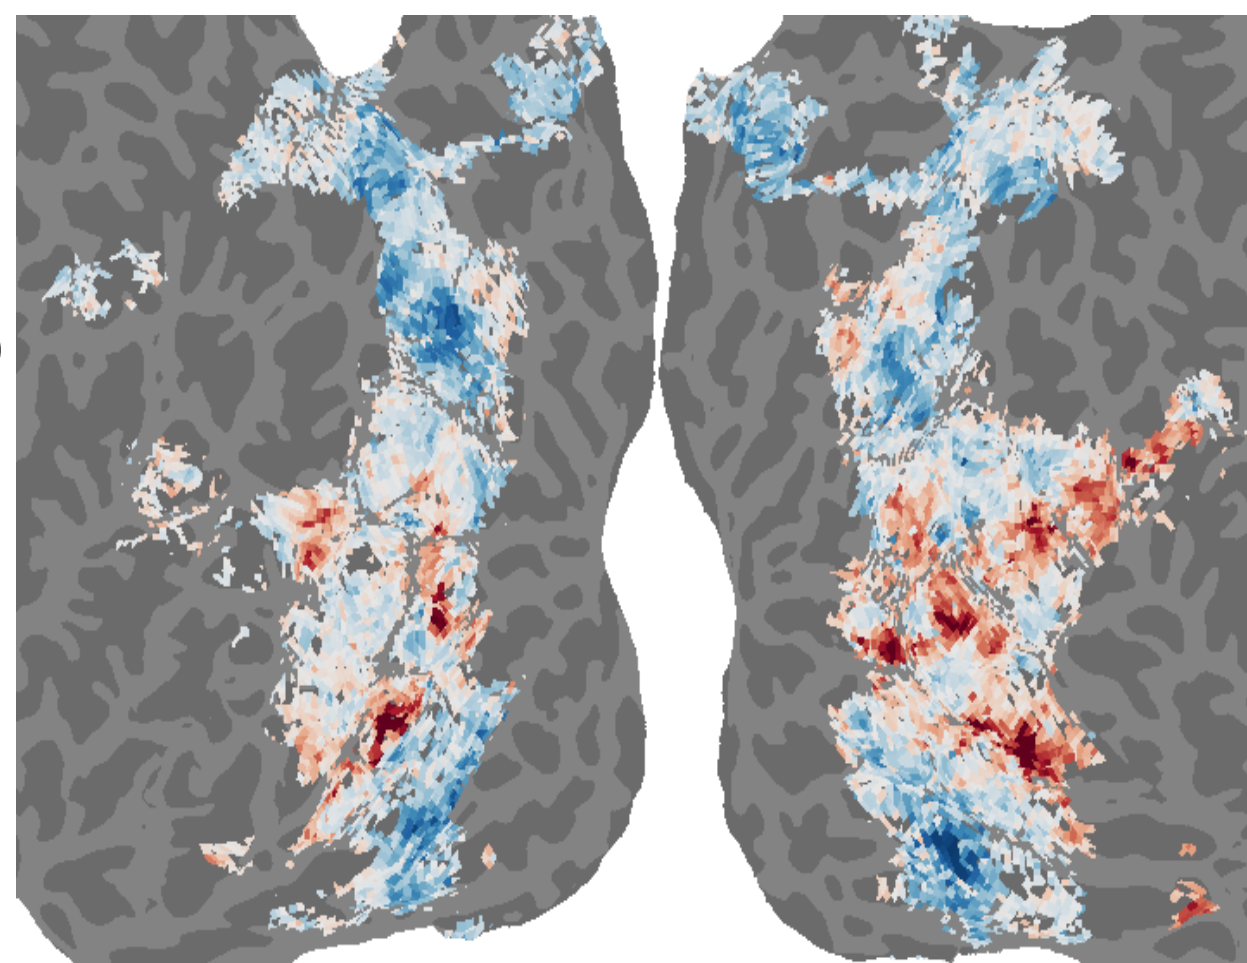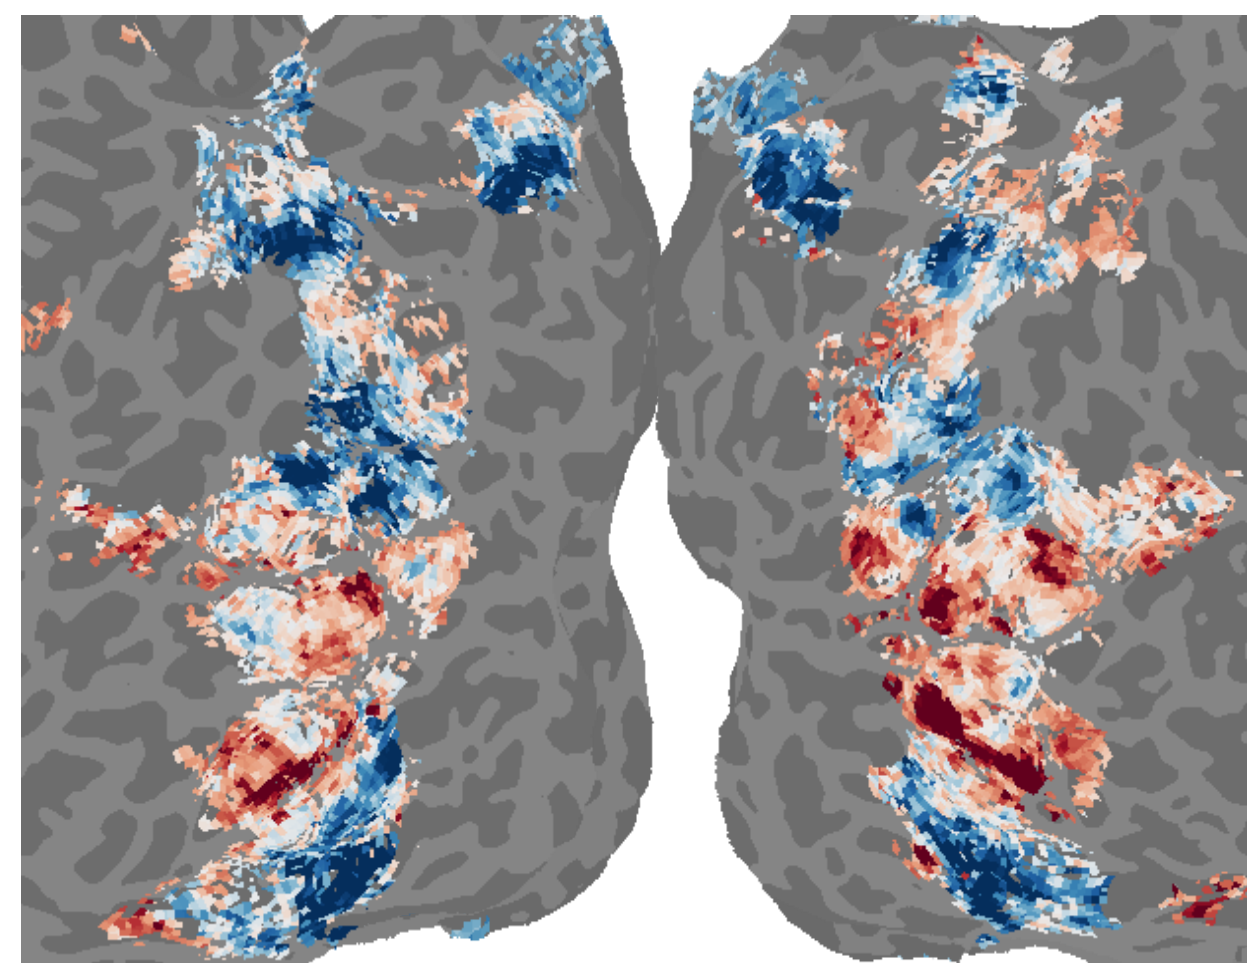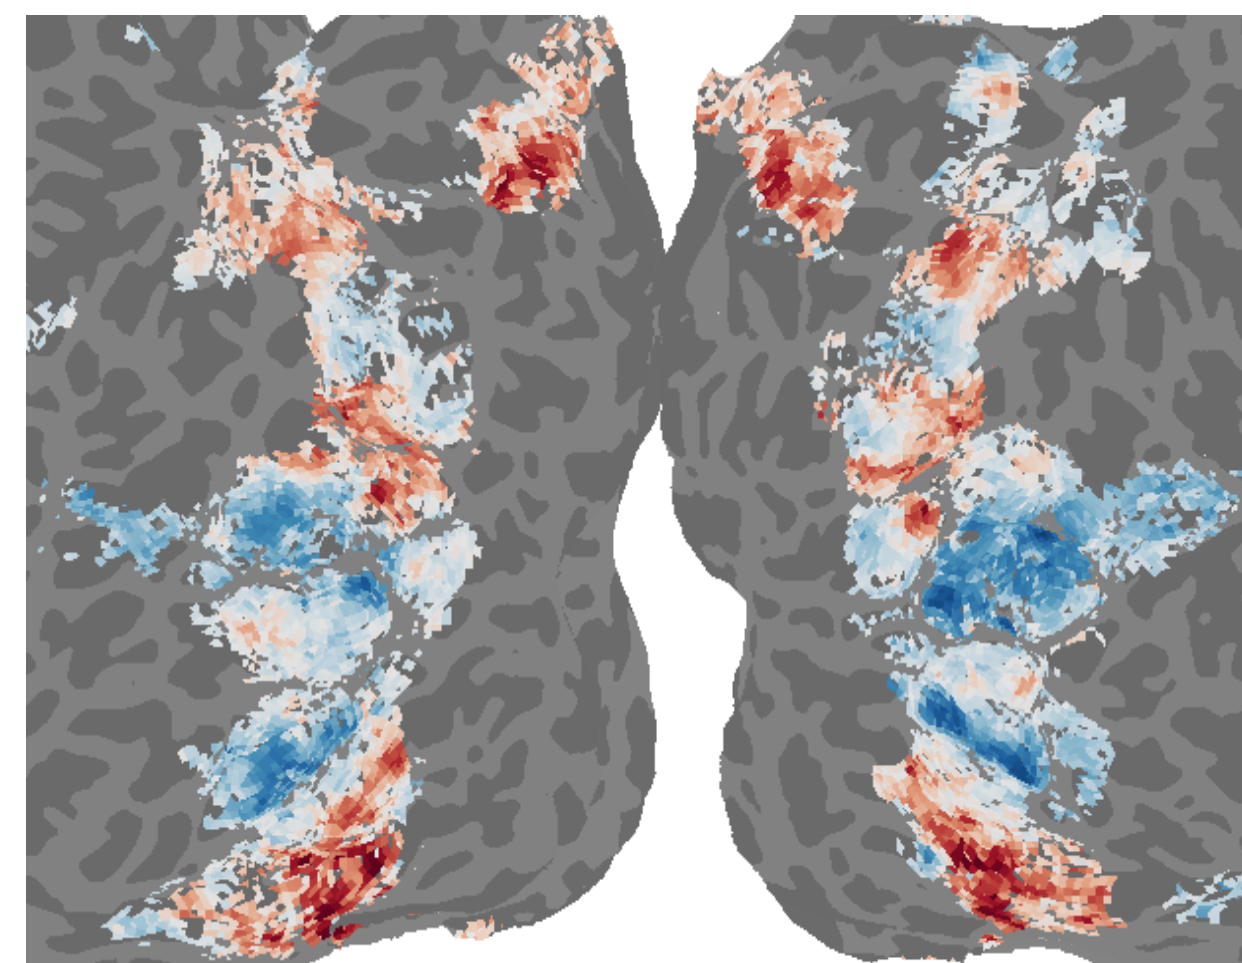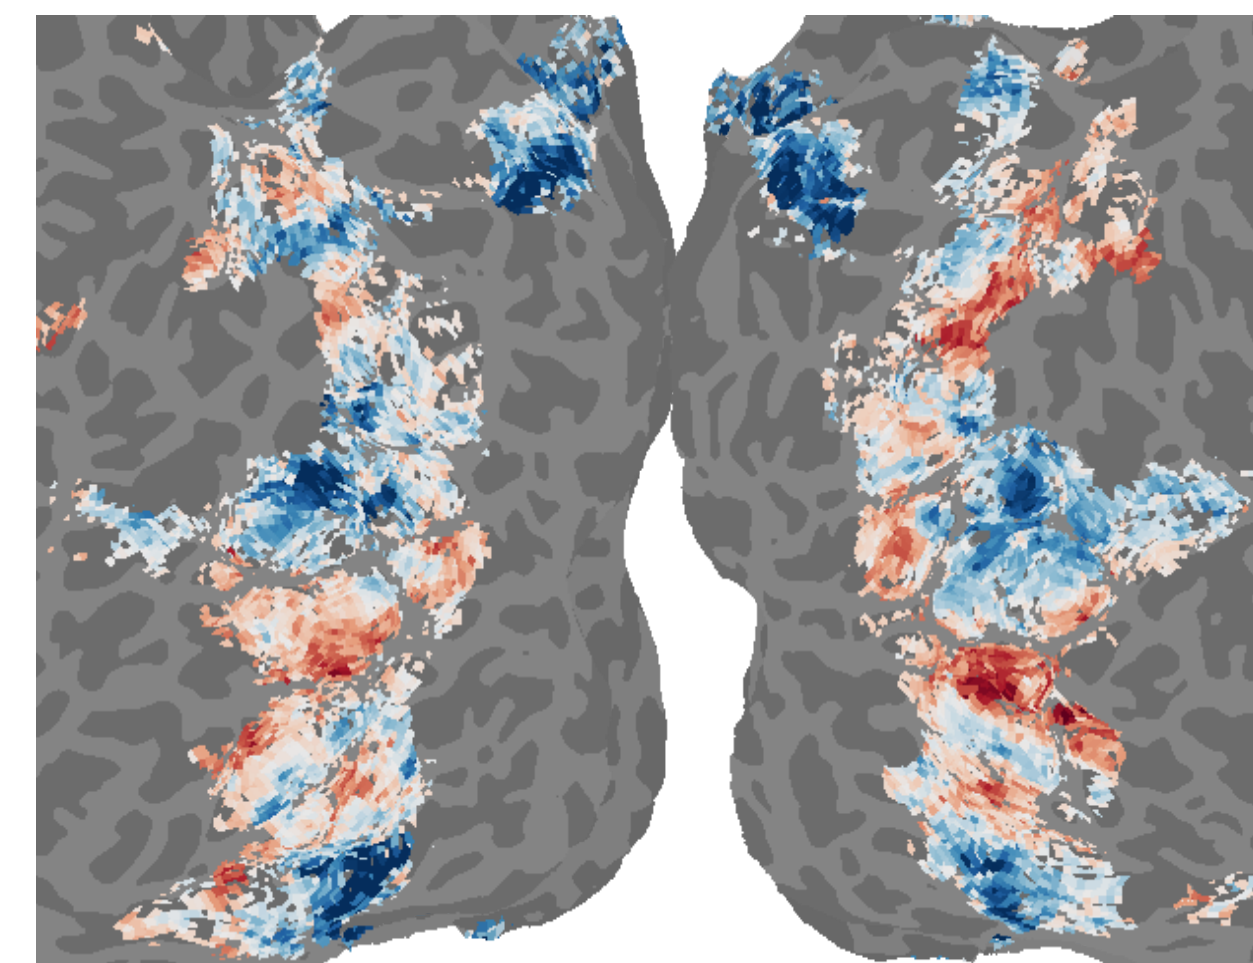

“A photo of a torso”

“A photo of a person's face”

“A photo of a bedroom”

“A photo of words”



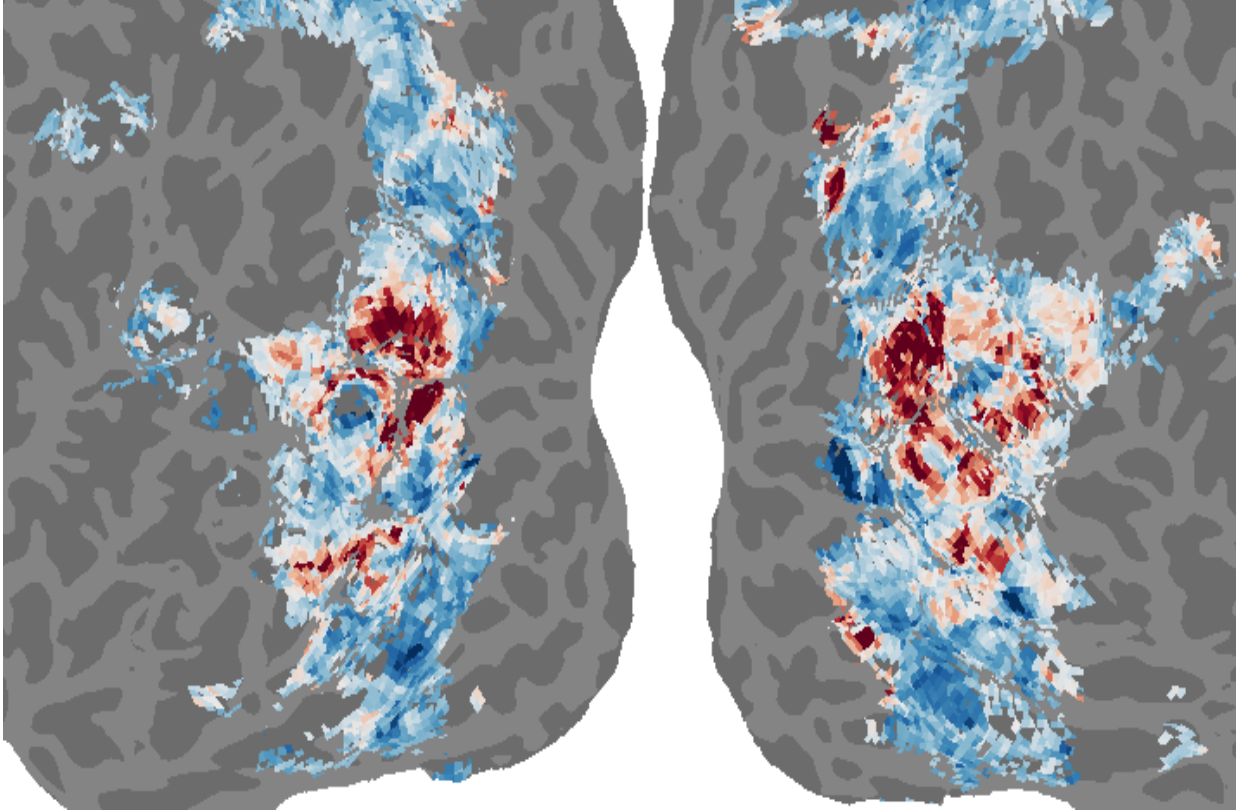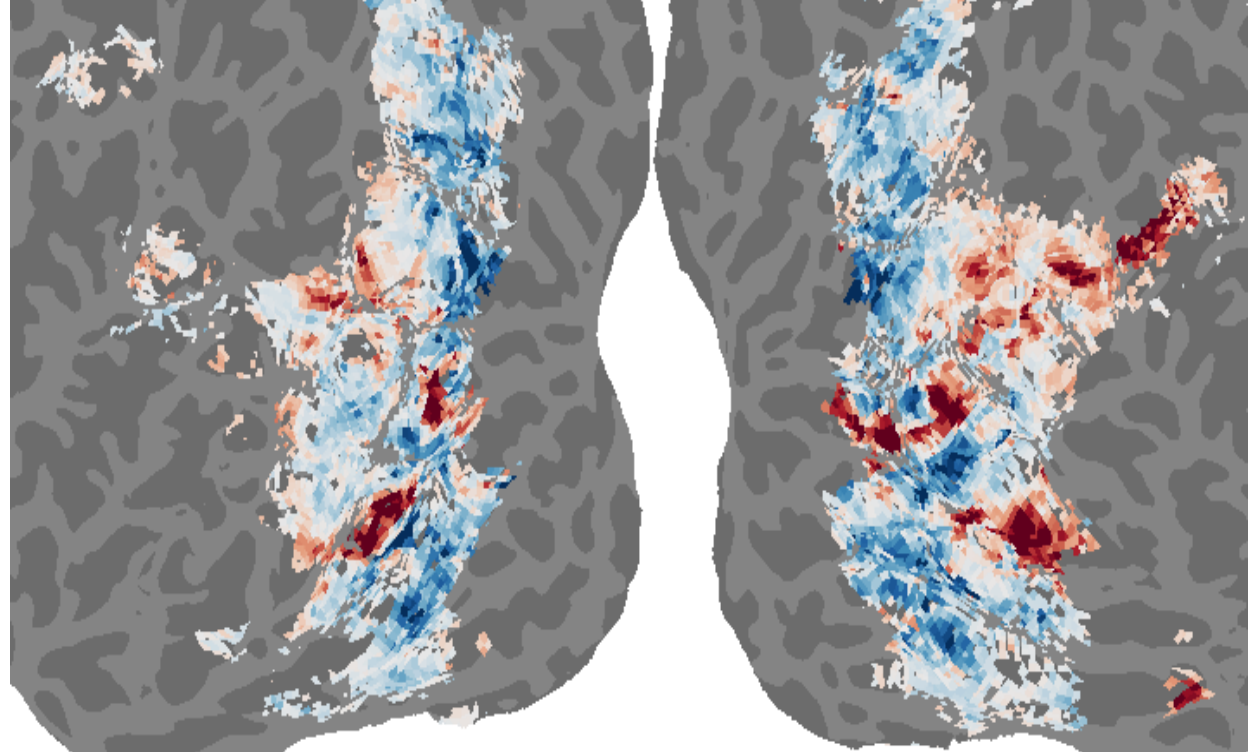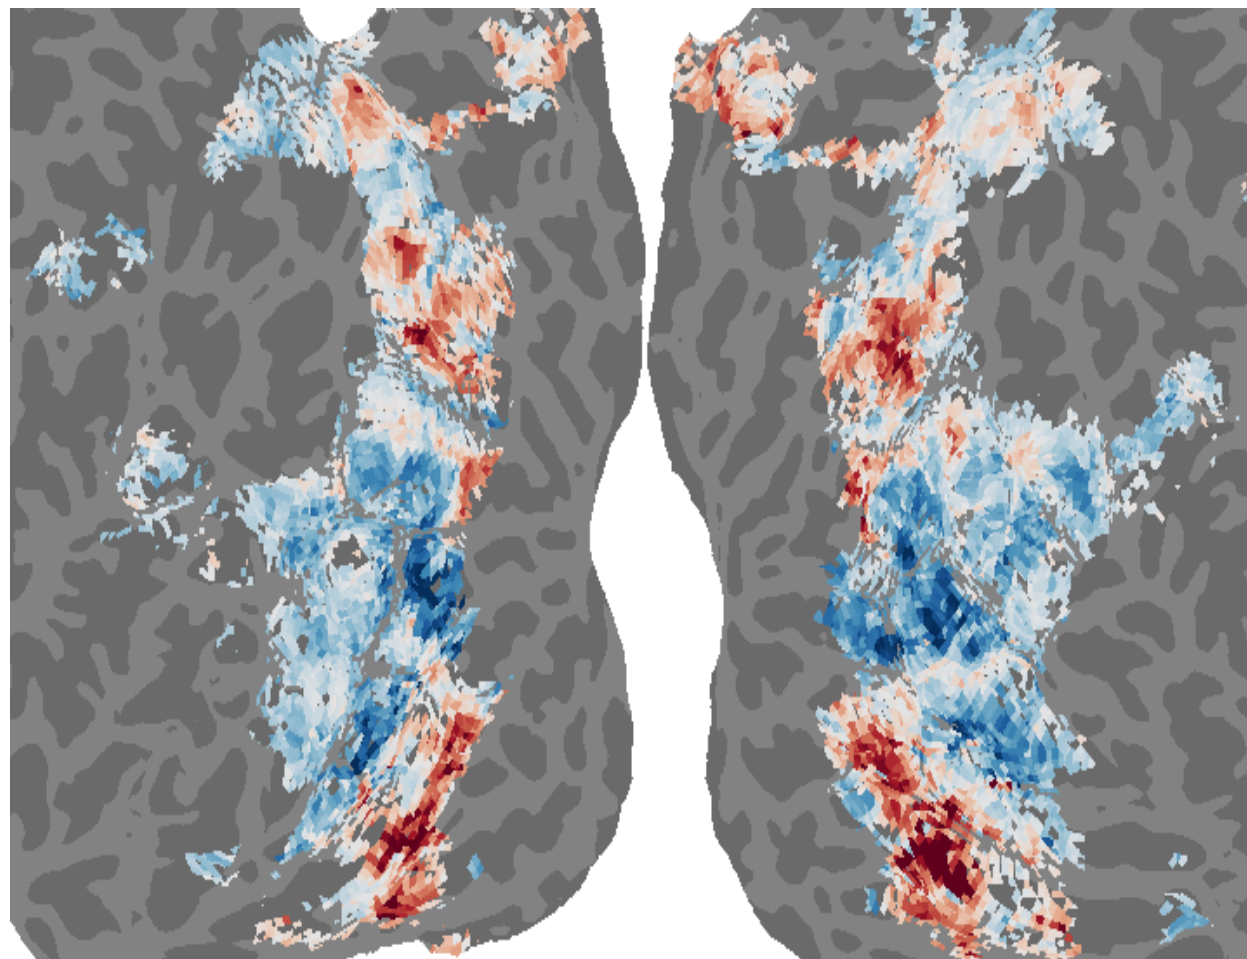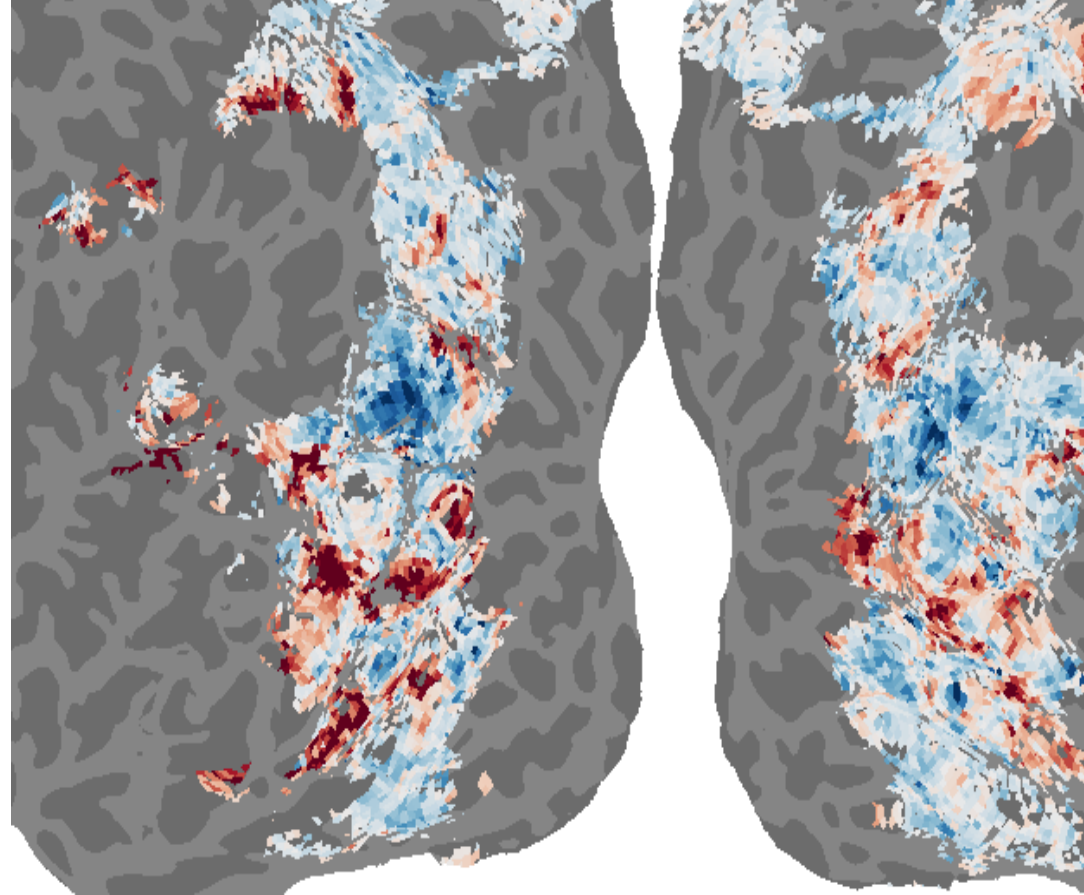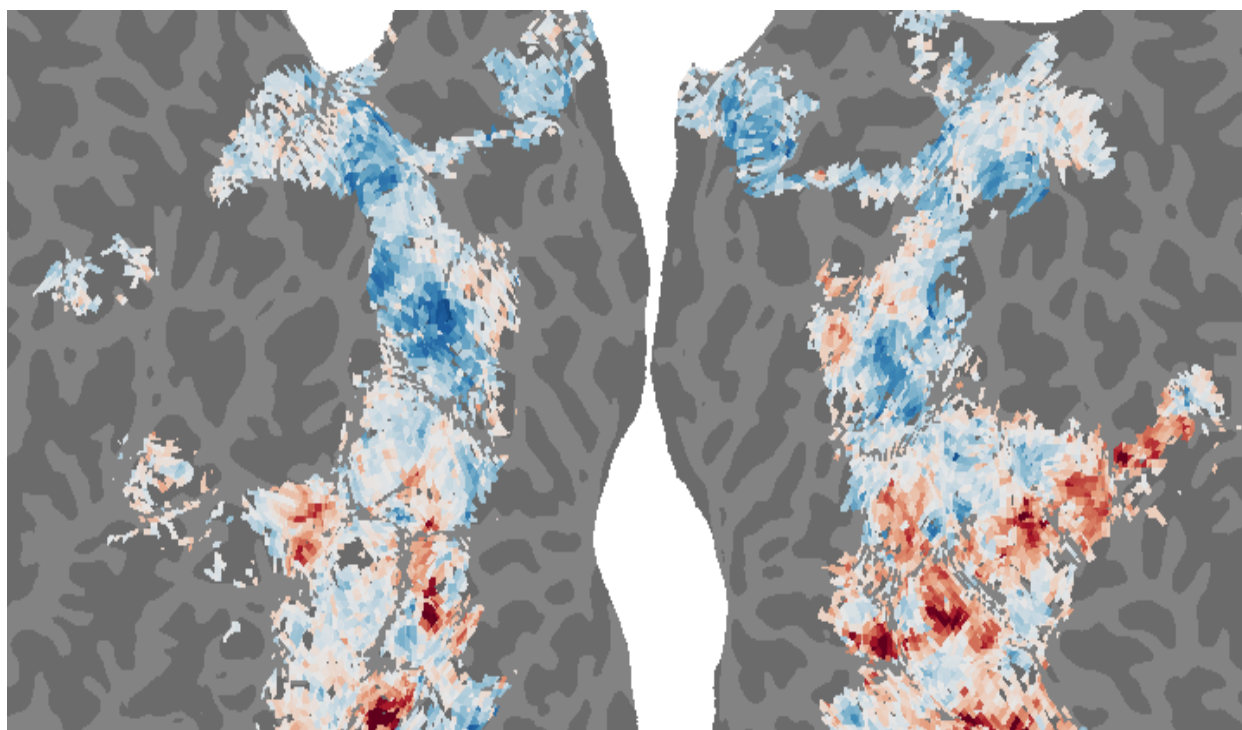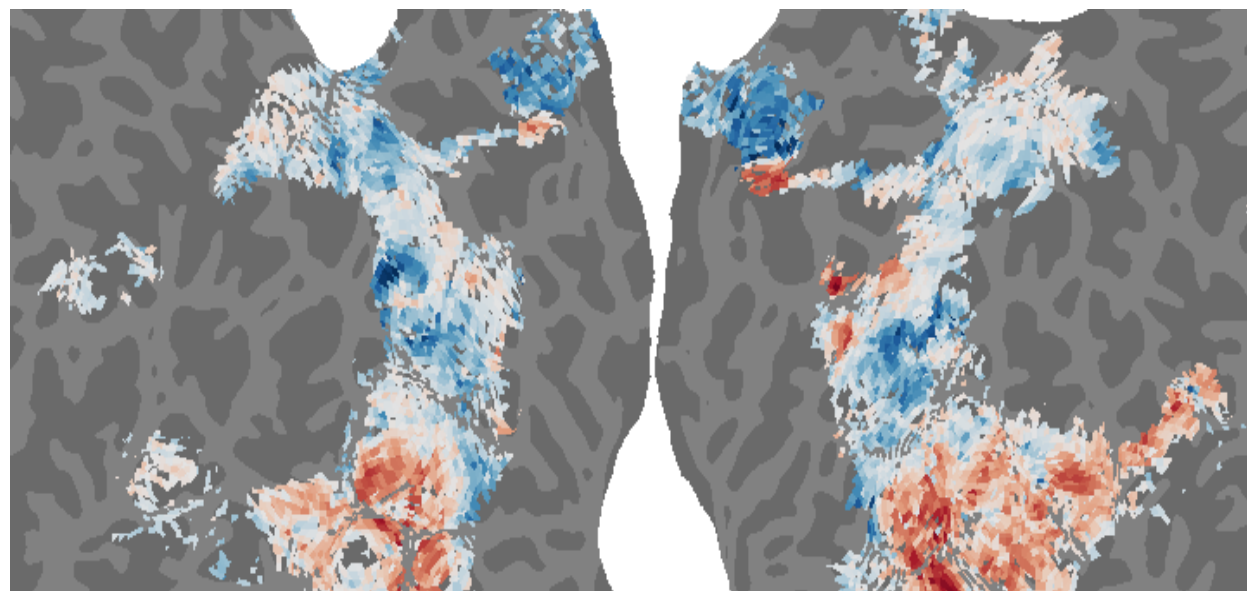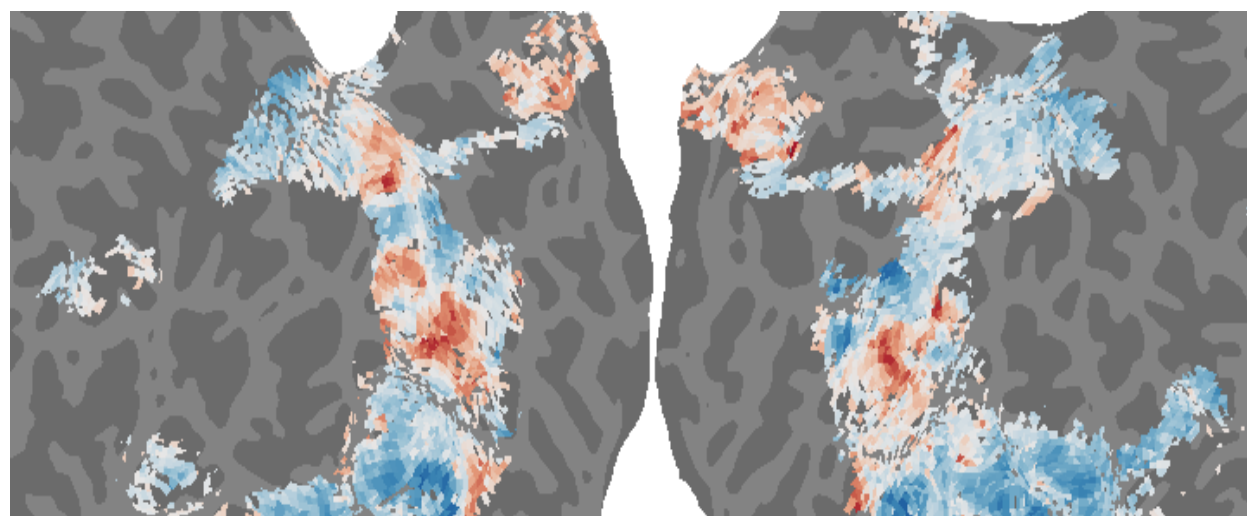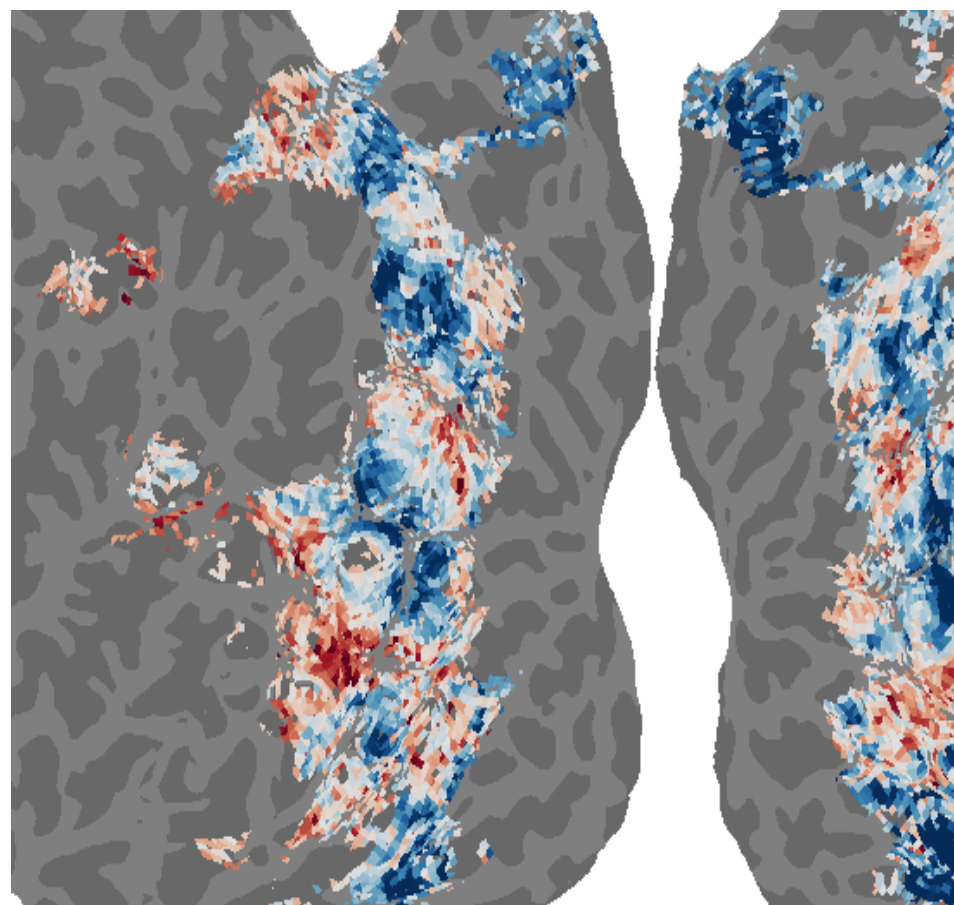

Supplement: Supplementary file 1 [file 11_probe_s6.pdf]
